# Supplementary material for: Forecasting Hands and Objects in Future Frames
Source: arXiv:1705.07328 source file (2018-08-23)
Supplement: Supplementary file 1 [file appendix.tex]

\begin{figure*}[t]
 \centering
    \includegraphics[width=1.0\textwidth]{figures/pr_curves_loc_1s}
    %\vspace{-3pt}
  \caption{Precision-recall curves of 1-sec future object location forecast results.}
 \label{fig:pr_curves_loc_1s}
    \includegraphics[width=1.0\textwidth]{figures/pr_curves_loc_5s}
    %\vspace{-3pt}
  \caption{Precision-recall curves of 5-sec future object location forecast results.}
 \label{fig:pr_curves_loc_5s}
 %\vspace{-6pt}
\end{figure*}
